# Supplementary material for: Graph Neural Networks for Improved El Ni\~no Forecasting
Source: arXiv:2012.01598 source file (2021-02-12)
Supplement: Supplementary file 1 [file 6_appendix.tex]

\section{Appendix}\blXX{todo: rewrite, contains redundant information and unreferenced text}
\begin{figure}[t]
 \centering
 \begin{subfigure}{1.\columnwidth}
  \centering
      \includegraphics [trim=0 0 0 0.1in, clip, width=1.\textwidth, angle = 0]{figures/100_florence_harvey}
      \vspace{.02in}
      %\caption{Before training}
  \end{subfigure}
\caption[Unconditioned model]{Generated post-flooding imagery of the first $100$ tiles of the hurricane Harvey (left) and hurricane Florence (right) test set. \blXX{todo: mention in appendix}} \label{fig:100_florence_harvey} 
\end{figure}
\subsection{Dataset}\label{sec:appendix_dataset}
\subsubsection{Pre- and post-flood imagery}
Post-flood images that display standing water are challenging to acquire due to cloud-cover, time of standing flood, satellite revisit rate, and cost of high-resolution imagery. The xBD is the best publicly available data-source for high-resolution imagery of pre- and post-flood images at the time of writing (see Appendix or~\cite{Gupta_2019}.  
\begin{itemize}
    \item Data Overview: $3284$ flood-related image pairs from seven flood events at 1024x1024px of ~0.5m/px resolution of which 30\% display a standing flood (~1370)
    \item Flood-related events: hurricanes (Harvey, Florence, Michael, Matthew), spring floods (Midwest US, ‘19), tsunami (Indonesia), monsoon (Nepal)
    \item Our evaluation test set is composed by 108 images of hurricane Harvey, 108 of hurricane Florence. The test set excludes imagery from hurricane Michael or Matthew, because the majority of tiles does not display standing flood. % 98 of Hurricane Michael, and 73 of hurricane Matthew.
\end{itemize}
\subsubsection{Flood segmentations}
\blXX{Describe how flood segmentations have been created.}
For $\sim 100$ post-flood images, manually annotated segmentation masks of flooded/non-flooded pixels have been created. The labelled imagery will be made available at the project gitlab.

\subsubsection{Storm Surge predictions}
Developed by the National Weather Service (NWS), the Sea, Lake and Overland Surges from Hurricanes (SLOSH) model~\cite{Jelesnianski_92} estimates storm surge heights from atmospheric pressure, size, forward speed and track data, which are used as a wind model driving the storm surge. The SLOSH model consists of shallow water equations, which consider unique geographic locations, features and geometries. The model is run in deterministic, probabilistic and composite modes by various agencies for different purposes, including NOAA, National Hurricane Center (NHC) and NWS. We use outputs from the composite approach -- that is, running the model several thousand times with hypothetical hurricanes under different storm conditions. As a result, we obtain flood hazard map as displayed in (\cref{fig:related_works}, bot-left), “Storm Surge Prediction”, which are storm-surge, height-differentiated, flood extents. After implementing the SLOSH model into our workflow, we will use the state-of-the-art ADvanced CIRCulation model (ADCIRC)~\cite{Luettich_1992} model, which has a stronger physical foundation, better accuracy, and higher resolution than SLOSH. ADCIRC storm surge model output data is available for the USA from the Flood Factor online tool developed by First Street Foundation.

\subsection{Experiments}\label{sec:appendix_experiments}
Standard data augmentation, here rotation, random cropping, hue, and contrast variation \blXX{ask chris}, and state-of-the art augmentations target to satellite imagery, here elastic transformations (citation). Further spectral normalization has been used to ... And a relativistic loss function has been implemented to ... \blXX{TODO-table} shows the quantitative evaluation of these experiments, but shows the none of the experiments have increased performance. 
We trained Pix2pixhHD on LPIPS loss and not on physics-consistency loss (e.g., dice-sorensen, iou).

\textbf{Pre-training LPIPS on satellite imagery.} The standard LPIPS did not clearly distinguish in between the flood baseline and generated flood model, contrasting the opinion of a human evaluator. This is most likely because LPIPS currently leverages a neural network that was trained on object classification from ImageNet. The neural network might not be capable to extract meaningful high-level features to compare the similarity of satellite images. This was confirmed by preliminary tests in which the network would classify all satellite imagery as background image. Future work, will use LPIPS with a network trained to have satellite imagery specific features, e.g., Tile2Vec or a land-use segmentation~\cite{Robinson_2019} model. %Advanced: Modified FID with a feature space that is pretrained on a satellite imagery segmentation task, 
\blXX{add .. extending on~\cite{Zhou_2020}}

\blXX{todo:add thoughts on why high-res is necessary; add thought on climate change isn't v. visible}
